# Supplementary material for: Correlated transitions in TKE and mass distributions of fission fragments described by 4-D Langevin equation
Source: arXiv:1805.10889 source file (2018-12-24)
Supplement: Supplementary file 1 [file supplementary_info-systematic4d-scientific-reports.pdf]

# Supplementary Information for Article in $\langle$ SREP-18-31029 $\rangle$

## Correlated transitions in TKE and mass distributions of fission fragments described by 4-D Langevin equation

Mark D. Usang, Fedir A. Ivanyuk, Chikako Ishizuka and Satoshi Chiba.

### Tabulated Total Kinetic Energy (TKE) Data of Fissioning System.

This supplementary information for our paper on *Correlated transitions in TKE and mass distributions of fission fragments described by 4-D Langevin equation* are the data used in plotting Fig. 3 and Fig. 4. The nuclide calculated here are further analyzed for the rest of the results.

| $Z$ | $A$ | $Z^2 A^{-1/3}$ | $E_x$ | TKE <sub>asy</sub> | $N_{asy}$ | TKE <sub>sym</sub> | $N_{sym}$ | $\langle TKE \rangle$ |
|-----|-----|----------------|-------|--------------------|-----------|--------------------|-----------|-----------------------|
| 92  | 236 | 1369.63        | 20.0  | 174.99             | 90712     | 162.72             | 10610     | 173.57                |
| 93  | 234 | 1403.54        | 20.0  | 177.30             | 2334      | 167.81             | 525       | 175.24                |
| 93  | 235 | 1401.55        | 20.0  | 177.36             | 3438      | 166.70             | 680       | 175.22                |
| 93  | 236 | 1399.57        | 20.0  | 176.40             | 4466      | 167.01             | 812       | 175.21                |
| 93  | 237 | 1397.60        | 20.0  | 177.76             | 4788      | 167.03             | 658       | 176.30                |
| 93  | 238 | 1395.64        | 20.0  | 177.09             | 4432      | 166.02             | 494       | 175.70                |
| 93  | 239 | 1393.69        | 20.0  | 176.98             | 5222      | 166.72             | 540       | 175.56                |
| 93  | 240 | 1391.75        | 20.0  | 176.47             | 4990      | 165.54             | 496       | 175.45                |
| 94  | 236 | 1429.83        | 20.0  | 180.82             | 6360      | 172.17             | 1100      | 178.77                |
| 94  | 237 | 1427.81        | 20.0  | 180.84             | 6374      | 172.50             | 882       | 178.93                |
| 94  | 238 | 1425.81        | 20.0  | 180.27             | 8632      | 171.02             | 1160      | 178.41                |
| 95  | 239 | 1454.27        | 20.0  | 184.71             | 11034     | 174.27             | 1323      | 182.34                |
| 95  | 240 | 1452.25        | 20.0  | 184.26             | 9286      | 176.13             | 780       | 182.32                |
| 95  | 241 | 1450.24        | 20.0  | 183.42             | 9990      | 174.59             | 689       | 181.59                |
| 95  | 242 | 1448.24        | 20.0  | 182.72             | 7978      | 174.37             | 598       | 181.65                |
| 95  | 243 | 1446.25        | 20.0  | 183.06             | 7958      | 175.09             | 455       | 181.40                |
| 96  | 243 | 1476.86        | 20.0  | 186.36             | 13362     | 177.83             | 1969      | 185.18                |
| 96  | 244 | 1474.84        | 20.0  | 186.46             | 13962     | 179.45             | 1974      | 184.80                |
| 96  | 245 | 1472.83        | 20.0  | 185.60             | 9554      | 179.00             | 1347      | 184.16                |
| 97  | 244 | 1505.72        | 20.0  | 189.79             | 10768     | 183.81             | 1062      | 188.04                |
| 97  | 245 | 1503.67        | 20.0  | 189.54             | 10618     | 182.37             | 950       | 187.84                |
| 97  | 246 | 1501.63        | 20.0  | 189.49             | 8330      | 182.18             | 756       | 187.64                |
| 97  | 247 | 1499.60        | 20.0  | 188.51             | 8440      | 182.97             | 495       | 187.29                |
| 98  | 245 | 1534.84        | 20.0  | 193.08             | 18712     | 187.87             | 2565      | 191.47                |
| 98  | 246 | 1532.75        | 20.0  | 192.22             | 13868     | 186.65             | 1850      | 190.83                |
| 98  | 247 | 1530.68        | 20.0  | 191.92             | 10360     | 186.88             | 1293      | 190.68                |
| 98  | 248 | 1528.62        | 20.0  | 192.16             | 10490     | 188.10             | 1338      | 190.26                |
| 98  | 249 | 1526.57        | 20.0  | 191.69             | 7288      | 186.62             | 941       | 190.26                |
| 98  | 250 | 1524.53        | 20.0  | 189.88             | 8978      | 187.78             | 1602      | 189.88                |
| 99  | 254 | 1547.60        | 8.0   | 196.52             | 269138    | 229.11             | 4910      | 197.39                |
| 100 | 256 | 1574.90        | 7.2   | 196.63             | 378838    | 226.63             | 46014     | 200.01                |
| 100 | 257 | 1572.85        | 7.0   | 197.59             | 407186    | 232.71             | 67130     | 202.55                |
| 100 | 258 | 1570.82        | 7.5   | 198.48             | 101214    | 234.48             | 298650    | 226.17                |
| 100 | 259 | 1568.79        | 8.0   | 196.19             | 218742    | 234.15             | 415066    | 221.06                |
| 101 | 260 | 1598.27        | 8.0   | 199.07             | 188972    | 238.54             | 454580    | 226.69                |

|     |     |         |     |        |        |        |        |        |
|-----|-----|---------|-----|--------|--------|--------|--------|--------|
| 102 | 256 | 1638.52 | 7.0 | 205.46 | 256684 | 235.26 | 37180  | 208.95 |
| 102 | 258 | 1634.28 | 7.0 | 204.83 | 335112 | 240.04 | 105840 | 213.43 |
| 103 | 259 | 1664.33 | 7.0 | 208.17 | 341838 | 240.57 | 45972  | 211.13 |
| 104 | 258 | 1699.00 | 7.0 | 213.54 | 251500 | 240.98 | 27298  | 217.17 |
| 104 | 260 | 1694.63 | 7.0 | 212.68 | 312390 | 244.44 | 77920  | 220.20 |

In this table, the variable  $Z$ ,  $A$  and  $E_x$  denotes respectively the charge, mass and excitation energy associated with the nuclide in question. The fissioning system  $Z^2 A^{-1/3}$  of the fissioning nucleus is related to the Coulomb repulsion of fission fragments. The quantities  $\text{TKE}_{\text{asy}}$  and  $\text{TKE}_{\text{sym}}$ , are the TKE associated respectively with asymmetric and symmetric mass splits. The numbers of fission events ending up with the asymmetric and symmetric mass splits in our calculations are given by  $N_{\text{asy}}$  and  $N_{\text{sym}}$  respectively from which we determine the dominant fission modes. The average TKE,  $\langle \text{TKE} \rangle$  is calculated by taking the sum of the TKE for each fission event and dividing it with the total number of fission events.

The calculations for the isotopes with  $Z$  number between 92 to 98 are done with  $E_x = 20$  MeV. The fission calculations with Langevin equation at such low excitation energy are quite common and they are equivalent to the excitation energy of fission events by the incident 14 MeV neutrons. At higher  $Z$  number, the neutron induced fission data are quite scarce but spontaneous fission data are quite abundant. The initial excitation energy in spontaneous fission should be close to zero but the fission calculations with Langevin equation with zero excitation is impossible. The system would never cross the fission barrier. Thus, we start our calculation with the lowest excitation energy. One can see from the table that for  $Z$  number beyond 98, the excitation energy of most isotopes is between 7 and 8 MeV.
